# Supplementary material for: OOD-HOI: Text-Driven 3D Whole-Body Human-Object Interactions Generation Beyond Training Domains
Source: arXiv:2411.18660 source file (2024-11-27)
Supplement: Supplementary file 1 [file X_suppl.tex]

\clearpage
\setcounter{page}{1}
\maketitlesupplementary

% \section{Rationale}
% \label{sec:rationale}
% % 
% Having the supplementary compiled together with the main paper means that:
% % 
% \begin{itemize}
% \item The supplementary can back-reference sections of the main paper, for example, we can refer to \cref{sec:coarse generation};
% \item The main paper can forward reference sub-sections within the supplementary explicitly (e.g. referring to a particular experiment); 
% \item When submitted to arXiv, the supplementary will already included at the end of the paper.
% \end{itemize}
% % 
% To split the supplementary pages from the main paper, you can use \href{https://support.apple.com/en-ca/guide/preview/prvw11793/mac#:~:text=Delete%20a%20page%20from%20a,or%20choose%20Edit%20%3E%20Delete).}{Preview (on macOS)}, \href{https://www.adobe.com/acrobat/how-to/delete-pages-from-pdf.html#:~:text=Choose%20%E2%80%9CTools%E2%80%9D%20%3E%20%E2%80%9COrganize,or%20pages%20from%20the%20file.}{Adobe Acrobat} (on all OSs), as well as \href{https://superuser.com/questions/517986/is-it-possible-to-delete-some-pages-of-a-pdf-document}{command line tools}.

% Our method generates 3D whole-body human-object interaction poses from textual prompts, considering the relative object point clouds and the contact areas between the hands and the object. However, the diversity of objects and actions in the dataset remains limited, constraining the model's generalization ability for broader practical application scenarios. 

In this supplementary material, we provide detailed descriptions of the text annotation process, along with data summaries, experimental details, dynamic adaptation specifics, and the network architectures utilized in our pipeline. We also present additional views of qualitative results with failure cases and discuss limitations and future work. For further results including qualitative comparisons and additional video demonstrations, please refer to the accompanying supplementary video.

\section{Dataset}
\subsection{Text Prompt Annotation}

Since the GRAB dataset~\cite{taheri2020grab} does not provide text prompts that describe the human-object interactions, collecting such prompts is necessary to facilitate the generation of 3D human-object interactions from text prompts. Text prompts should include details about the interacting hand type (e.g., left hand, right hand, or both), the action involved (e.g., lift, pass, place), and the object category or name (e.g., apple, airplane, bowl). The basic format for text prompts is as follows: \textit{\{action\} \{object category\} with \{hand type\}} (e.g., \textit{Pass airplane with right hand}). We automatically annotate text using the provided action labels, which include both the action and the object category. However, these labels do not specify the interacting hand type. We determine the interacting hand type based on the proximity between the hand and the object in global 3D space: if the distance during interaction is less than a predefined threshold (5~mm), we consider the hand to be involved in the interaction.

\subsection{Stable Poses}

Our \mymethod{OOD-HOI} mainly focus on generating stable grasp poses. To ensure high-quality data, we collect frames where the hand demonstrates a stable grasp and remove those without close contact. To select stable pose frames for training \textbf{\mymethod{OOD-HOI}}, we adopt the following criteria, inspired by GrabNet~\cite{taheri2020grab}:

\begin{enumerate}
    \item The hand must be in contact with the object.
    \item The object's vertical position must differ by at least 5~mm from its initial position (i.e., the object should be lifted off the resting surface).
    \item The interacting hand must have its thumb and at least one additional finger in contact with the object.
\end{enumerate}

Since the original GRAB dataset contains instances of interpenetration during contact, we apply an offset to address this issue. The offset is measured by the mean Chamfer distance between the pre-labeled body contact area and the object contact area, and it is applied to the human body translation during training. By applying these filters, we ensure that the dataset consists solely of stable grasps, which are essential for effectively training \mymethod{OOD-HOI}. Additionally, this dataset provides SMPLH~\cite{MANO:SIGGRAPHASIA:2017} parameters, object meshes, and information on object rotation and translation.

\section{Experimental Details}
\subsection{Implementation Details}

Both our dual-branch reciprocal diffusion model and the contact predictor are built on the Transformer architecture~\cite{vaswani2017attention} with 4 attention heads, a latent dimension of 512, a dropout rate of 0.1, a feed-forward size of 1024, and the GeLU activation function~\cite{hendrycks2016gaussian}. Similar to MDM~\cite{tevet2023human}, we employ the CLIP model~\cite{radford2021learning} to encode text prompts, adhering to a classifier-free generation process. Our models are trained on four NVIDIA A30 GPUs. Our training setup involves 20k iterations for the dual-branch reciprocal diffusion model and 10k iterations for the contact predictor. These iterations utilize a batch size of 512 and employ the AdamW optimizer~\cite{loshchilov2017decoupled} with a learning rate set at $10^{-4}$. We use $T_1 = 1000$ and $T_2 = 500$ diffusion steps in the dual-branch reciprocal diffusion model and the contact predictor, respectively.

\subsection{Training the action classifier}
We train a standard RNN action recognition classifier on the GRAB dataset and use the final layer of the classifier as the motion feature extractor for calculating action recognition accuracies as well as diversity (DIV) and multimodality (MM) scores, following IMoS~\cite{ghosh2022imos}. We employ the online available code from IMoS and use the same network architecture and parameters to train our model.  

\subsection{Additional Details of Evaluation Metrics}
For detailed information regarding metrics employed in human-object interaction pose generation, including \textit{Accuracy}, \textit{FID}, \textit{Diversity}, \textit{Multimodality}, we refer reader to~\cite{guo2022generating, tevet2023human} for comprehensive understanding.

Expanding on the concept of the interaction between human and object, we utilize \textit{Intersect Volume} metric to quantify the closeness between human hand joints and the object surface. To measure this, we voxelize the hand and object using a voxel size of 0.5cm. If the hand and the object collide, the penetration depth is the maximum of the distances from hand mesh vertices to the object surface.

\begin{figure}[!tbp]
\centering
\includegraphics[width=0.48\textwidth, trim=10cm 2cm 10cm 2cm, clip]{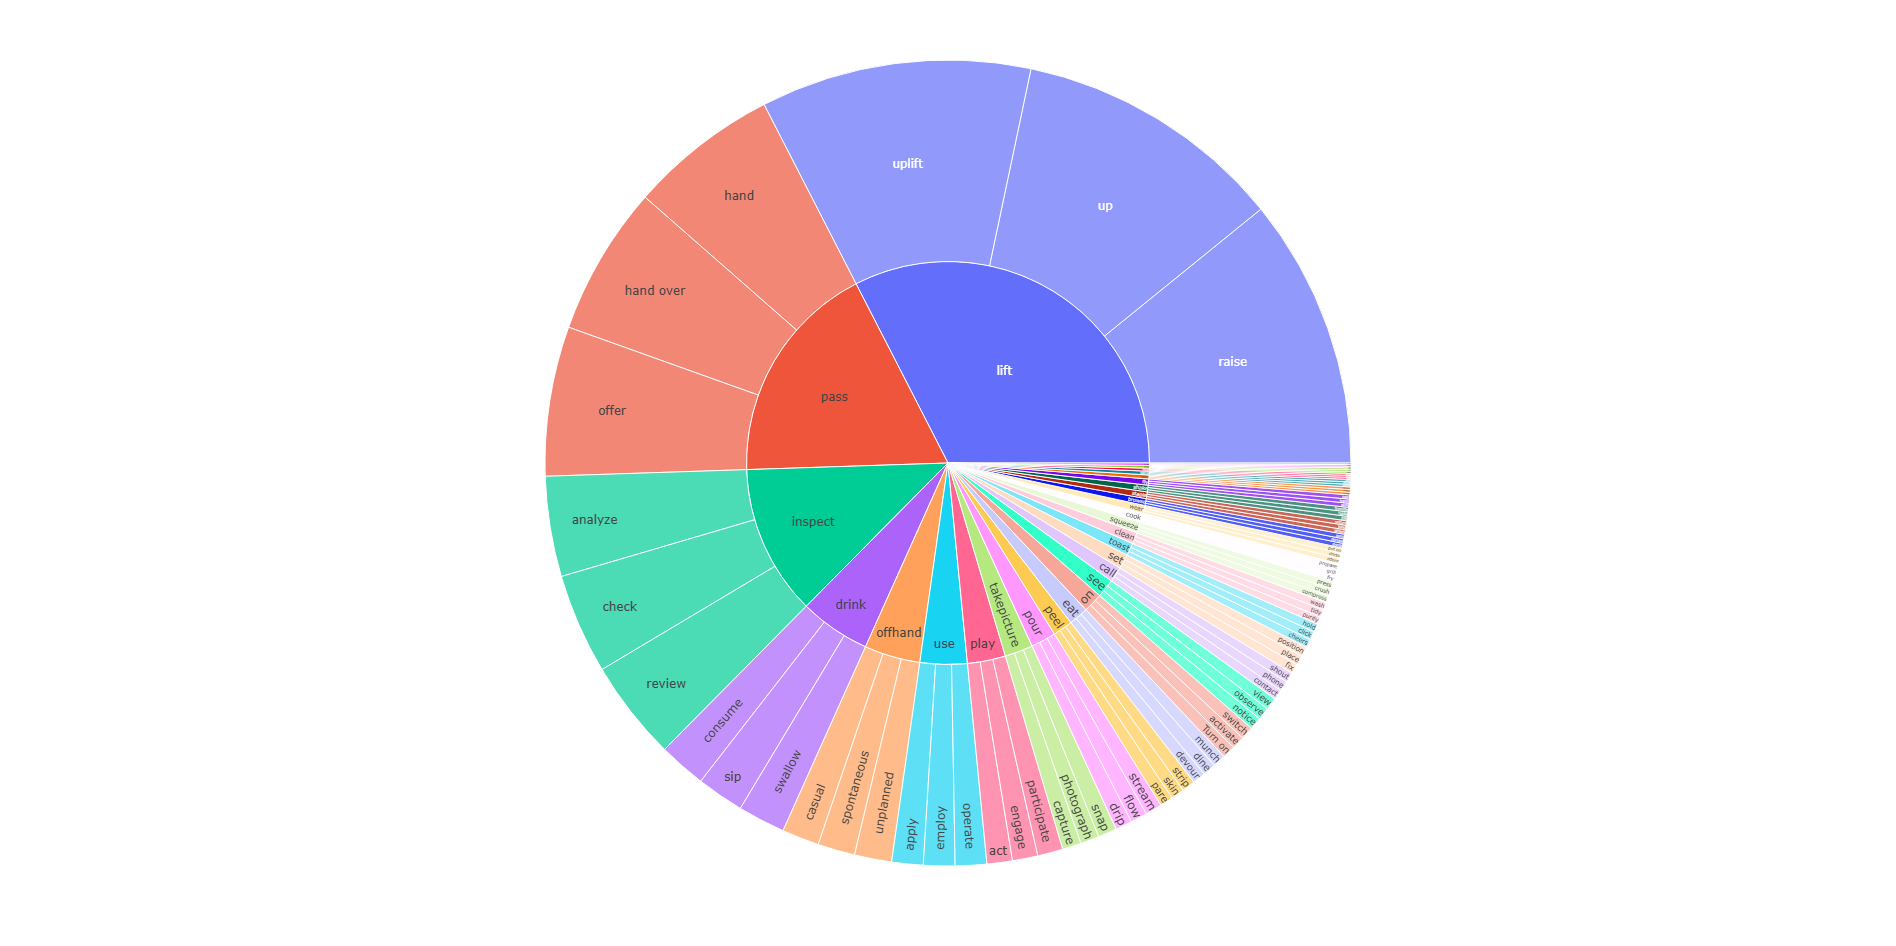}
\caption{Examples of annotated textual descriptions with semantic adjustments for the Grab dataset were generated using GPT-4o. The original actions (represented in the inner circle) are matched with their corresponding synonymous actions (shown in the outer circle), enriching the dataset's semantic diversity. The proportions reflect the frequency of each action's occurrence within the data. As a result of these semantic adjustments, the total number of actions increased significantly, expanding from 29 to 116.}
\label{fig:text_domain}
% \vspace{-.5em}
\end{figure}

\section{Dynamic Adaptation Details}
The GRAB dataset~\cite{taheri2020grab} consists of 51 distinct objects of varying shape and size with 29 action labels. Using these object and action labels, and identifying which hand is interacting with the object, We apply dynamic adaptation to enlarge the dataset for out-of-domain (OOD) generation.

\subsection{Semantic Adjustment}
For text-OOD generation, we introduce semantic adjustments to enhance the diversity of input text semantics. Table~\ref{fig:text_domain} shows a selection of annotated textual descriptions with semantic modifications for the GRAB dataset. The first row represents the original action annotation from the GRAB dataset, while the subsequent rows provide synonym-based alternatives. Through these semantic adjustments, the total number of action annotations increases to 116, effectively generating three synonyms for each original action label.

\subsection{Geometry Deformation}
For object-OOD generation, we apply geometric deformations to enhance the diversity of geometric representations. Figure~\ref{fig:geometry_deformation} illustrates a selection of deformed object geometries under constraints from the GRAB dataset. The first row shows the original object with its possible contact area highlighted in purple, while the rest rows display plausible deformed objects with random stretch and rotation applied to the non-contact areas. By applying these geometric deformations, the total number of objects increases from 51 to 204, with each object being deformed into three distinct alternative shapes. This process effectively enhances the diversity of geometric representations.

\begin{figure*}[!tbp]
\centering
\includegraphics[width=\textwidth, trim=0cm 0.5cm 1cm 0.5cm, clip]{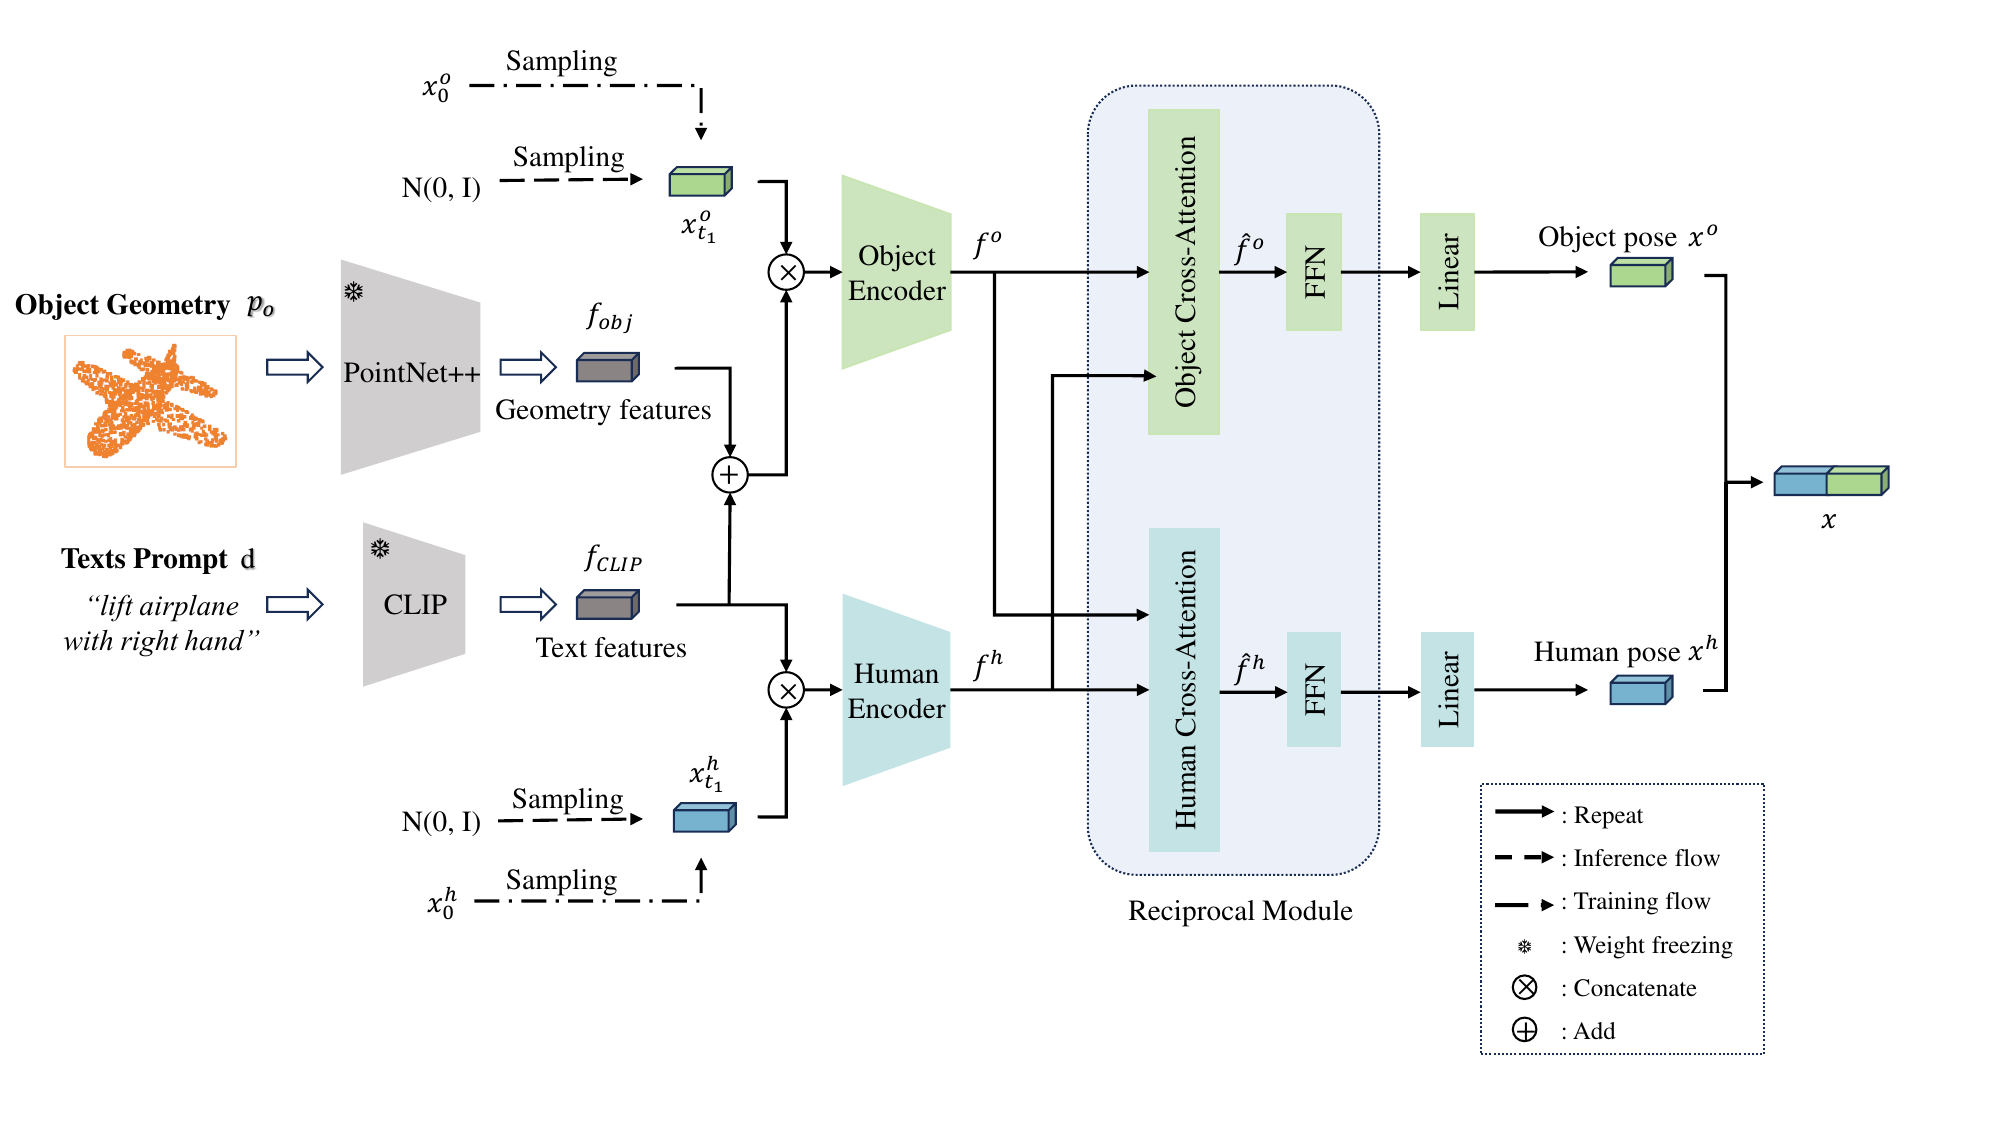}
\caption{Overview of Dual-Branch Reciprocal Diffusion Model. The model mainly consists of two branches: one for predicting object pose(shown in the green area) and another for predicting human pose(shown in the blue area). The object pose branch takes Gaussian random noise, object geometry features and textual features as inputs to predict the object pose. The human pose branch takes Gaussian random noise and textual features as inputs to predict the human pose. The two branches exchange information through the Reciprocal Module to enhance the interaction between object pose and human pose.}
\label{fig:dual_branch}
% \vspace{-.5em}
\end{figure*}

\section{Networks}
To generate plausible whole-body interaction pose, our OOD-HOI propose two networks including dual-branch reciprocal diffusion model and contact predict diffusion model.
\subsection{Dual-Branch Reciprocal Diffusion Model}
We propose a dual-branch reciprocal diffusion model for 3D whole-body interaction pose generation based on a text prompt $d$ and object geometry point clouds $p_o$. The generation procedure consists of six steps, as illustrated in Fig.~\ref{fig:dual_branch}: 1) extracting object features from the object geometry, 2) extracting text features from the text prompt, 3) sampling Gaussian random noise vectors for the human and object 4) encoding the Gaussian noise vectors with the corresponding conditions, 5) exchanging information through a reciprocal module and 6) generating the human-object interaction pose.

Specifically, to extract geometric features, we utilize PointNet++~\cite{qi2017pointnet++}, which outputs object features $f_{obj} \in \mathbb{R}^{N \times 512}$, where $N$ corresponds to the sampled points ($N=256$) and 512 represents the feature dimensions. For text features, the CLIP~\cite{radford2021learning} text encoder extracts $f_{CLIP} \in \mathbb{R}^{512}$ from the text prompt.

At training time, the object vector $x_{t_1}^o \in \mathbb{R}^6$ is sampled from the original object pose $x_0^o$, and the human vector $x_{t_1}^h \in \mathbb{R}^{159}$ is sampled from the original human pose $x_0^h$. At inference time, these vectors are sampled from a Gaussian distribution. Given the corresponding conditions (geometry features $f_{obj}$ and text features $f_{CLIP}$), the object vector $x_{t_1}^o$ is concatenated with $f_{obj}$ and $f_{CLIP}$ to form the object encoder features $f^o$. Similarly, the human encoder features $f^h$ are obtained by combining the human vector $x_{t_1}^h$ with $f_{CLIP}$.

To facilitate information exchange between $f^o$ and $f^h$, the reciprocal module employs a cross-attention mechanism. Specifically, the object output features $\hat{f}^o$ are generated using $f^o$ as the query and $f^h$ as the memory. A similar process is applied to obtain the human output features $\hat{f}^h$. Finally, the object pose $x^o$ is generated through feed-forward layers followed by a linear transformation, with a similar process used to generate the human pose $x^h$.

\begin{figure*}[!tbp]
\centering
\includegraphics[width=\textwidth, trim=0cm 1.5cm 4cm 1cm, clip]{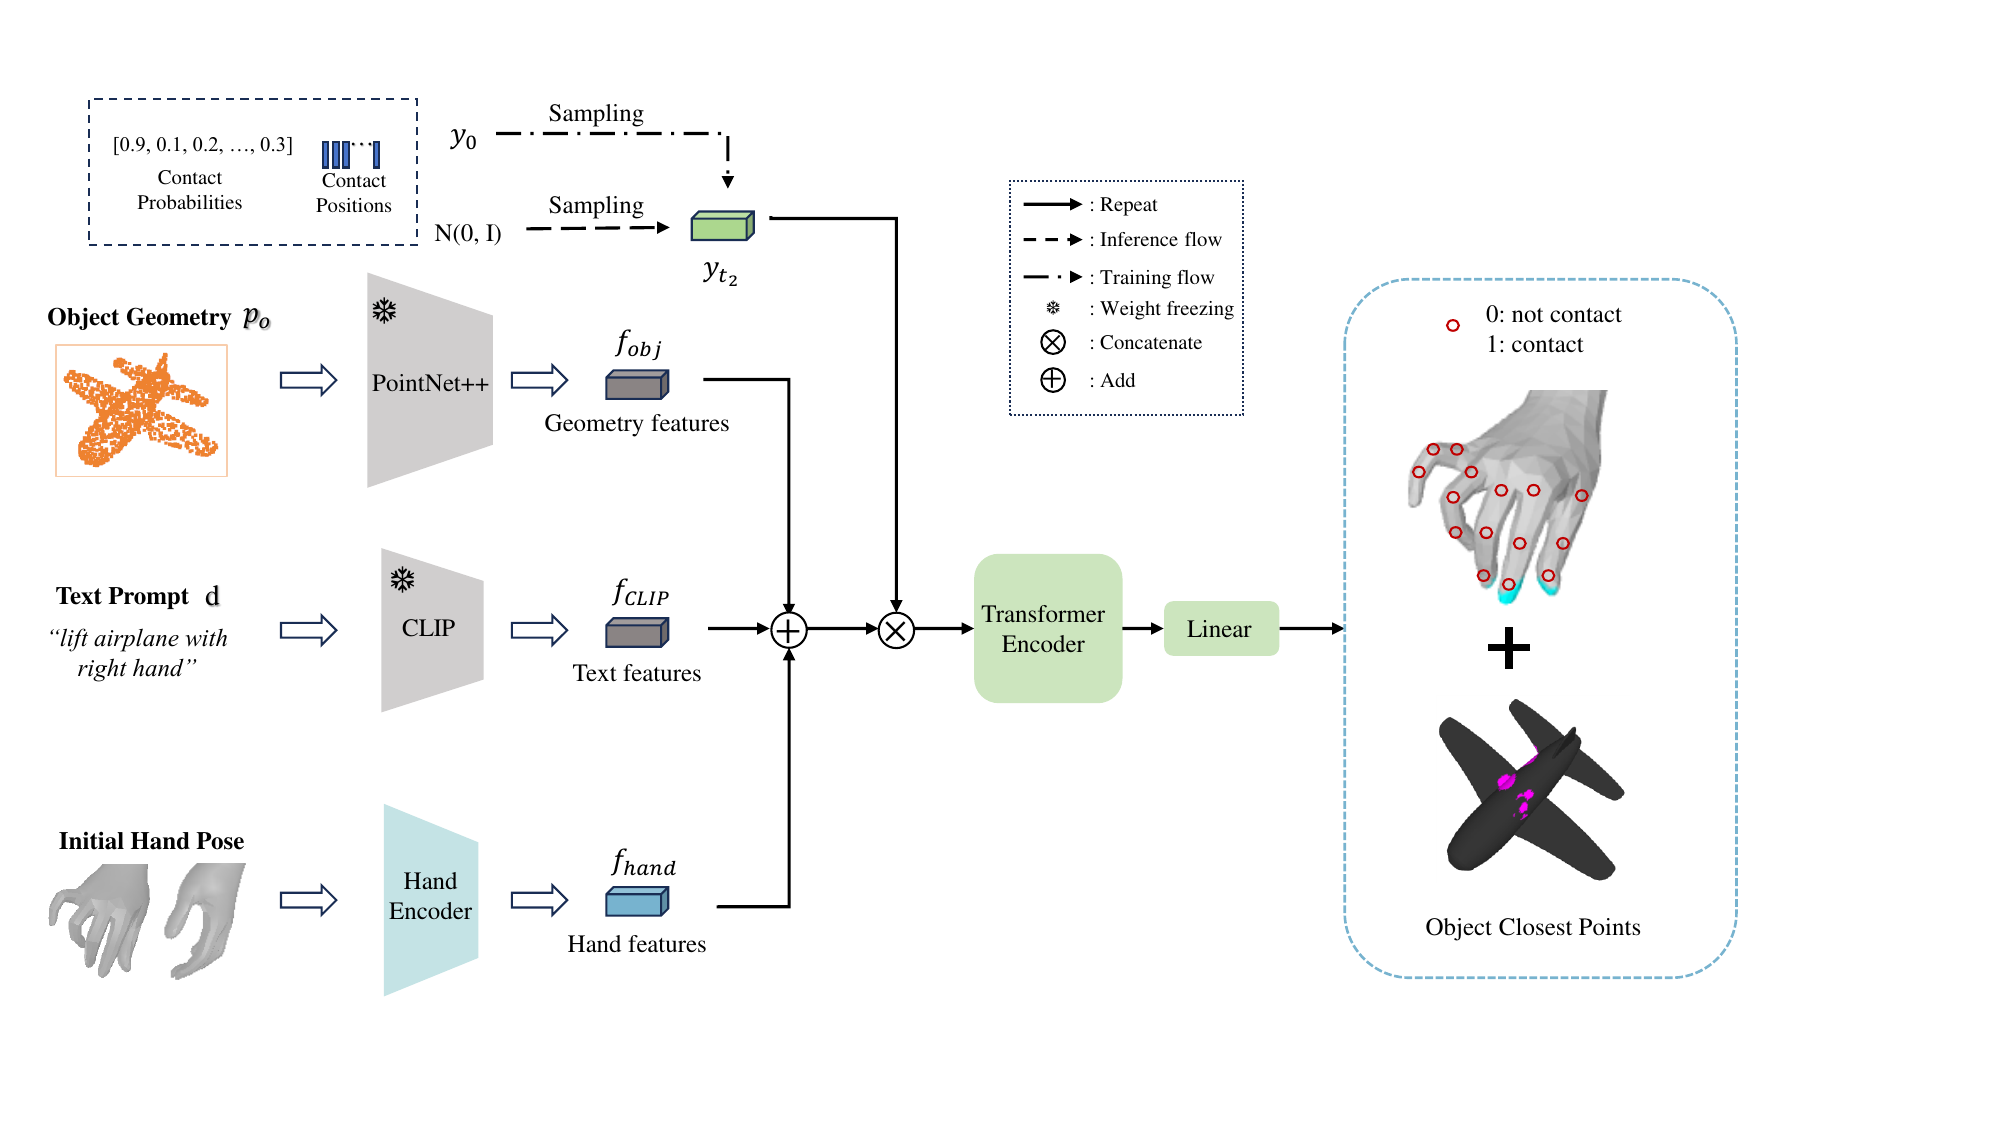}
\caption{Overview of Contact Predictor Diffusion Model. The Contact Predictor Diffusion Model predicts hand contact joints and their associated probabilities using a combination of geometric and contextual inputs. The model leverages Gaussian random noise, object geometric features, textual features, and hand pose features as inputs. These are processed within a transformer encoder to generate predictions.The contact area is determined by identifying the closest points between the hand’s contact joints and the object’s point cloud, computed using the Chamfer distance. This approach enables precise localization of contact regions, aligning hand-object interactions effectively.}
\label{fig:contact_predictor}
% \vspace{-.5em}
\end{figure*}

\begin{figure*}[!tbp]
\centering
\includegraphics[width=\textwidth, trim=2cm 0.5cm 2.8cm 0cm, clip]{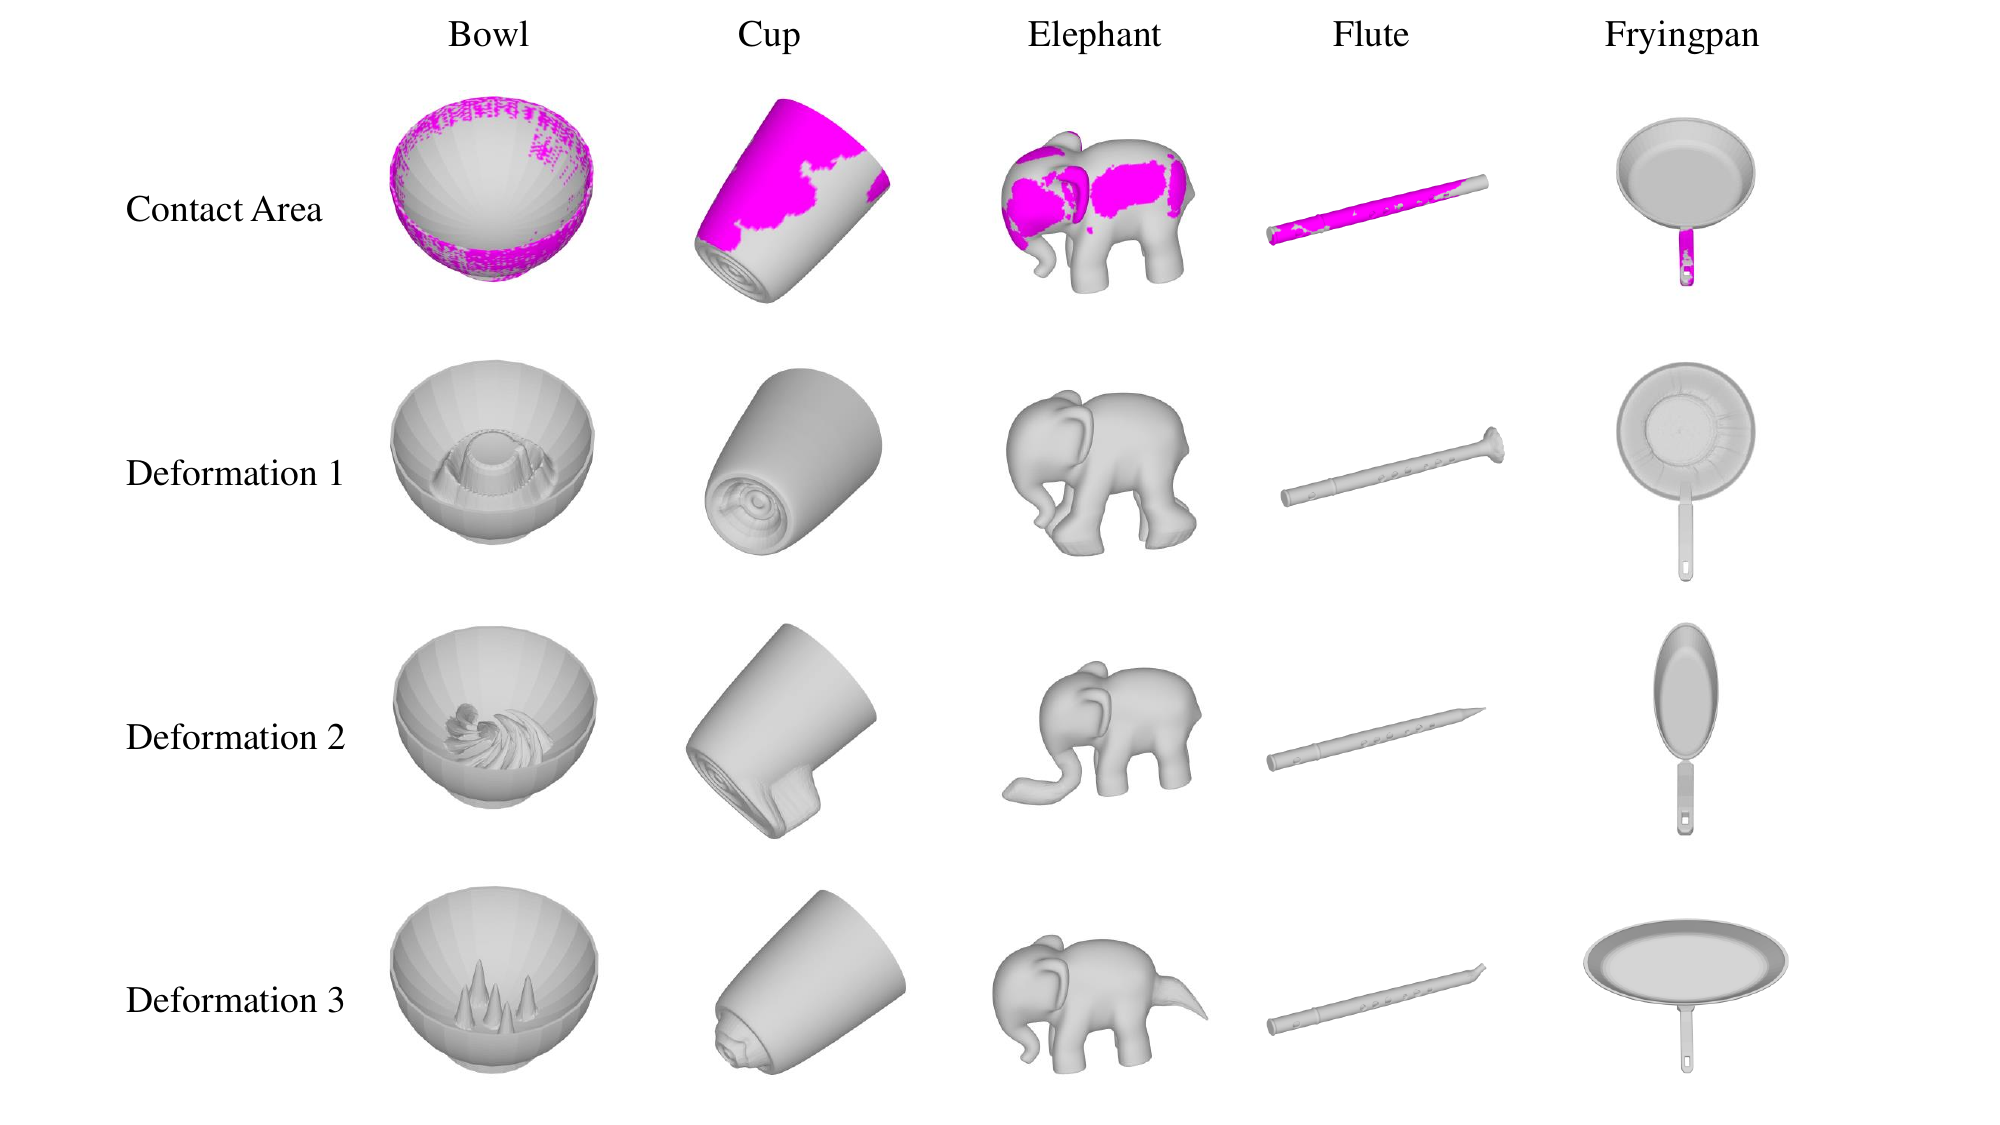}
\caption{Some Cases Using Geometry Deformation. We select \textit{bowl, cup, elephant, flute and fryingpan} as examples to demonstrate the effects of the proposed geometry deformation. The first row uses purple dots to show the annotated contact areas of the objects. The remaining rows display the objects' mesh after plausible deformation in non-contact areas.} 
\label{fig:geometry_deformation}
% \vspace{-.5em}
\end{figure*}

\subsection{Contact Predictor Diffusion Model}
Our contact predictor diffusion model takes several inputs, including object geometry point clouds $p_o$, text prompt $d$, the initial hand pose as a condition, and a noised contact vector $y_{t_2} \in \mathbb{R}^{30 \times 4}$ as input. The model outputs the denoised contact vector $y_0 \in \mathbb{R}^{30 \times 4}$, where $30$ represents two hand joints, and $4$ corresponds to the 3 axes of contact position along with 1 contact probability.

Similar to the dual-branch reciprocal diffusion model, the geometry features $f_{\text{obj}} \in \mathbb{R}^{N \times 512}$ are extracted using PointNet++, while the text features $f_{\text{CLIP}}$ are extracted using the CLIP text encoder. Additionally, the hand features $f_{\text{hand}} \in \mathbb{R}^{512}$ are obtained from a dedicated hand encoder, guided by an indicator function $\mathbf{H}$:

\[
\mathbf{H} =
\begin{cases}
    \{1, 0\}, & \text{if `left' appears in the text prompt}, \\
    \{0, 1\}, & \text{if `right' appears in the text prompt}, \\
    \{1, 1\}, & \text{if `both' appears in the text prompt}.
\end{cases}
\]

Specifically: if the text contains `left', only the left-hand features are added to the embedding, and right-hand features are excluded. Conversely, if the text contains `right', only the right-hand features are included. If the text contains `both', features for both hands are included in the embedding.

The contact predictor combines the geometry features $f_{\text{obj}}$, text features $f_{\text{CLIP}}$, and hand features $f_{\text{hand}}$ by adding them together. These combined features are then concatenated with the noised contact vector $y_{t_2}$ and passed through a Transformer encoder block. After applying a linear transformation, the model predicts the corresponding contact vector $y_0$. For the refiner, the object’s closest points are derived from the predicted contact vector to further refine the predictions.

\section{Qualitative Results and Failure Cases}
Fig. provides more viewpoints of our qualitative results. We see that most grasp look natural and plausible with right motion intent. More results with a rotating viewpoint are shown in the video.

OOD-HOI can still generate some failure cases (See Fig.). These are mostly cases of penetrating fingers and there are not many cases of contacting fingers that fly away from the object. Penetrations are observed mostly for objects with wrong predicted contact area (e.g., Grasp the mug with right hand with the predicted area is the bottom of the mug). Since the small amount of both hands interaction pose data, the generation of both hands pose is more likely to fail.
% Furthermore, we present three failure cases: the generated action dose not match the text prompt, the contact area is dose not match the text prompt, the hand in the text prompt is ignored.

\begin{figure*}[!tbp]
\centering
\includegraphics[width=\textwidth, trim=0cm 13cm 0cm 0cm, clip]{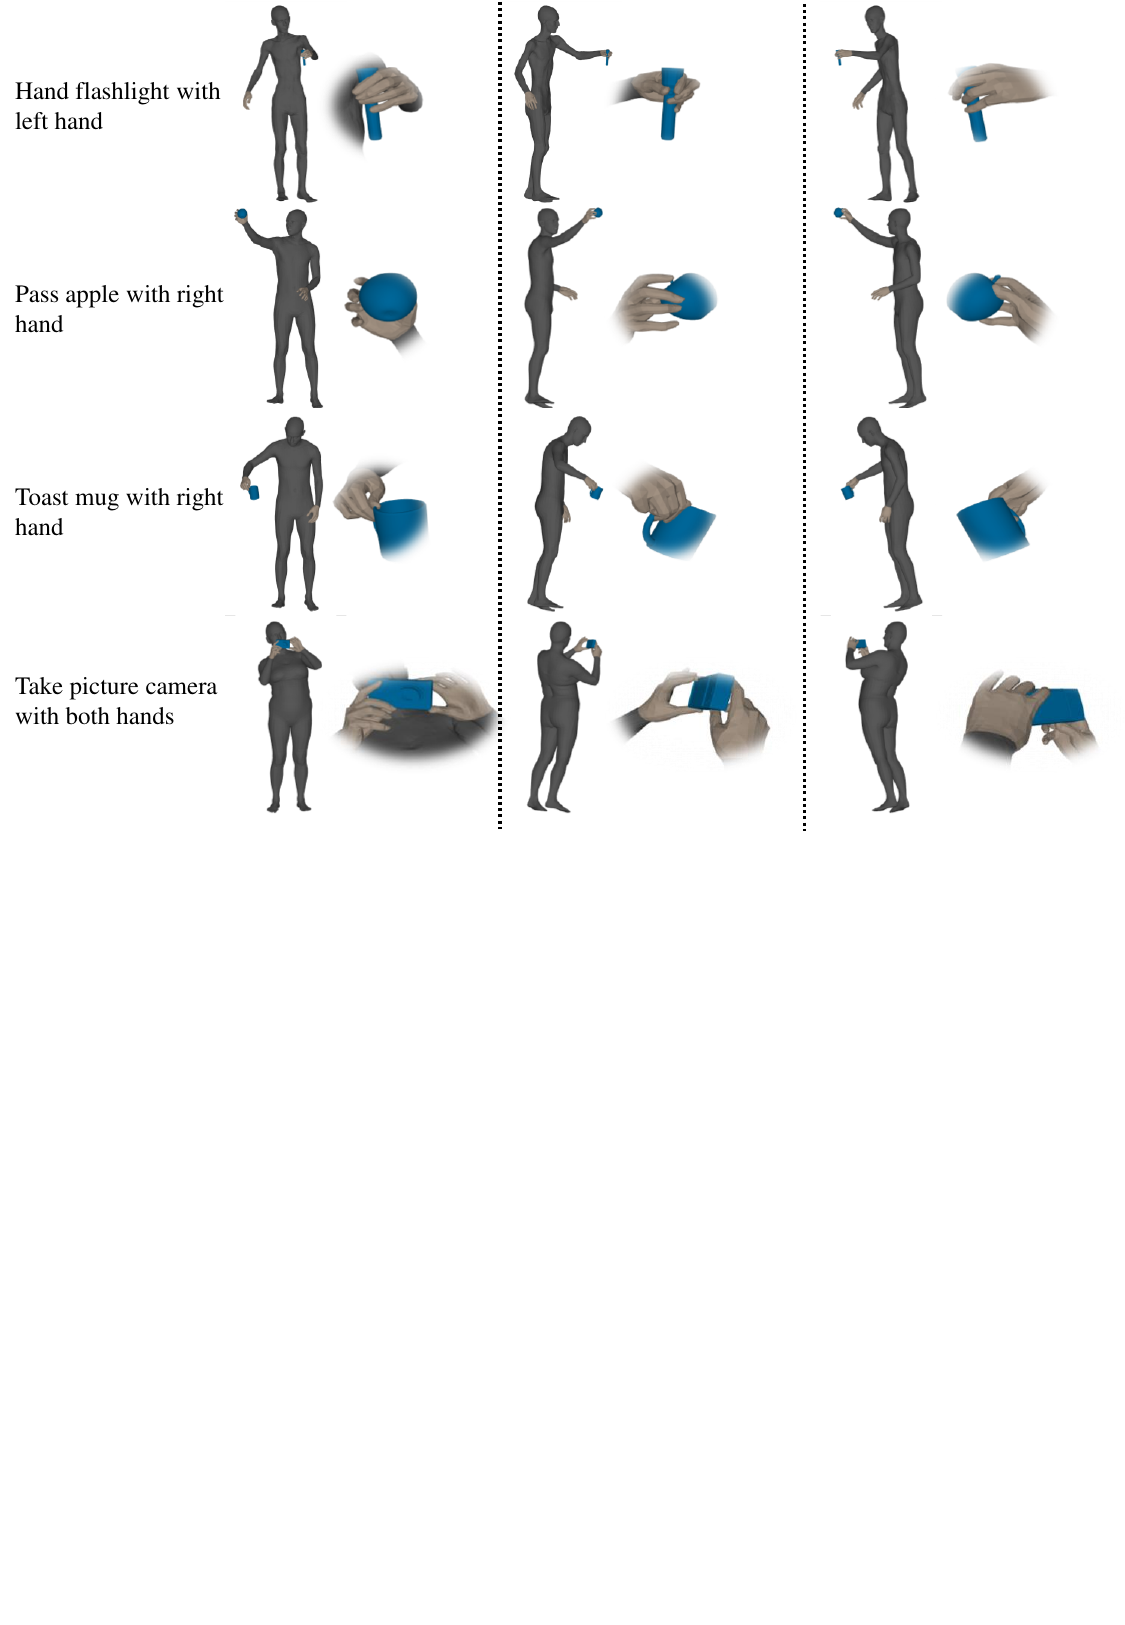}
\caption{In domain quantitative results for multi-view analysis. We present our results from three perspectives: front view, left view, and right view.}
\label{fig:multiview}
% \vspace{-.5em}
\end{figure*}

\begin{figure*}[!tbp]
\centering
\includegraphics[width=\textwidth, trim=0cm 6.5cm 0cm 3cm, clip]{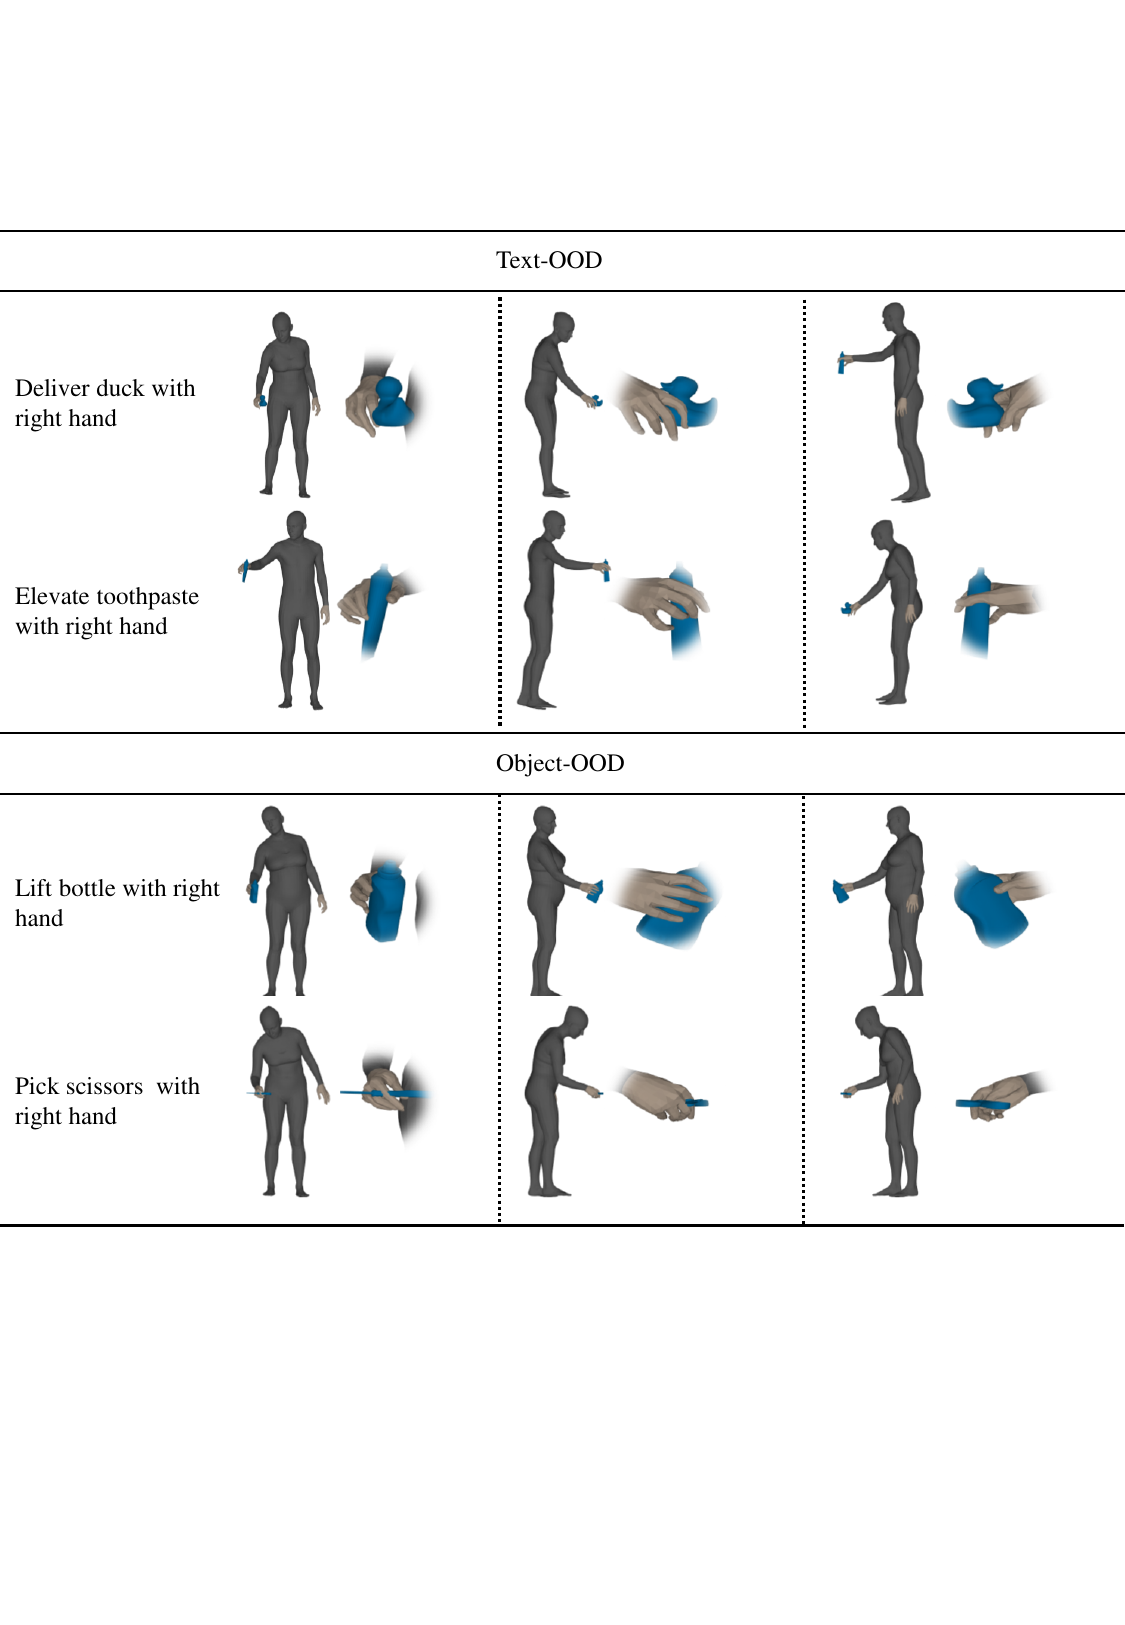}
\caption{Out-of-domain quantitative results for multi-view analysis. We present our results from three perspectives: front view, left view, and right view.}
\label{fig:outdomain_multiview}
% \vspace{-.5em}
\end{figure*}

\section{Limitation and Future Works}
Furthermore, while our approach focuses on generating static, stable grasp poses, practical applications often require generating dynamic human-object interaction motions directly from textual prompts. Addressing this limitation involves several challenges. Future work may focus on the following two aspects: 1) collecting a larger dataset of high-quality, 3D whole-body human-object interaction data from everyday life to enhance the diversity and realism of interactions. and 2) extending the model to generate human-object interaction motions, rather than static poses, based on textual prompts. This includes transitioning from static stable grasp poses to dynamic motions that align with the specified interactions. By addressing these challenges, the generation capability can be significantly improved, facilitating wider applicability in practical scenarios.
